# Supplementary material for: Homophily and Incentive Effects in Use of Algorithms
Source: arXiv:2205.09701 source file (2022-05-19)
Supplement: Supplementary file 1 [file appendix.tex]

\newpage 

\appendix

\section{Additional regression results}\label{sec:app_regresults}

\begin{table}[H] \centering 
  \caption{Regression results relative of OLS to estimate the impact of the interventions on participants' agreement fraction, switch fraction, and mean influence.} 
  \label{} 
\begin{tabular}{@{\extracolsep{5pt}}lD{.}{.}{-3} D{.}{.}{-3} D{.}{.}{-3} } 
\\[-1.8ex]\hline 
\hline \\[-1.8ex] 
 & \multicolumn{3}{c}{\textit{Dependent variable:}} \\ 
\cline{2-4} 
\\[-1.8ex] & \multicolumn{1}{c}{Agreement fraction} & \multicolumn{1}{c}{Switch fraction} & \multicolumn{1}{c}{Mean influence} \\ 
\\[-1.8ex] & \multicolumn{1}{c}{(1)} & \multicolumn{1}{c}{(2)} & \multicolumn{1}{c}{(3)}\\ 
\hline \\[-1.8ex] 
 \textit{Medium agreement} & 0.054^{*} & 0.146^{***} & 0.107^{**} \\ 
  & (0.031) & (0.054) & (0.047) \\ 
   \textit{High agreement} & 0.045 & 0.097^{*} & 0.114^{**} \\ 
  & (0.030) & (0.050) & (0.052) \\ 
  \textit{Medium agreement} $\times$ \textit{feedback} & -0.056 & -0.165^{***} & -0.136^{***} \\ 
  & (0.034) & (0.059) & (0.052) \\ 
  \textit{High agreement} $\times$ \textit{feedback} & -0.039 & -0.087 & -0.091 \\ 
  & (0.034) & (0.059) & (0.057) \\ 
  \textit{Neutral incentives} & 0.017 & 0.022 & 0.036 \\ 
  & (0.025) & (0.041) & (0.040) \\ 
  \textit{High-TP incentives} & 0.024 & 0.002 & 0.014 \\ 
  & (0.024) & (0.041) & (0.039) \\ 
  \textit{Intercept} & 0.701^{***} & 0.325^{***} & 0.264^{***} \\ 
  & (0.023) & (0.036) & (0.036) \\ 
 \hline \\[-1.8ex] 
Observations & \multicolumn{1}{c}{493} & \multicolumn{1}{c}{493} & \multicolumn{1}{c}{493} \\ 
R$^{2}$ & \multicolumn{1}{c}{0.013} & \multicolumn{1}{c}{0.028} & \multicolumn{1}{c}{0.027} \\ 
Adjusted R$^{2}$ & \multicolumn{1}{c}{0.001} & \multicolumn{1}{c}{0.016} & \multicolumn{1}{c}{0.015} \\ 
Residual Std. Error (df = 486) & \multicolumn{1}{c}{0.222} & \multicolumn{1}{c}{0.377} & \multicolumn{1}{c}{0.355} \\ 
\hline 
\hline \\[-1.8ex] 
\multicolumn{4}{l} {\parbox[t]{0.95\textwidth}{\footnotesize{ \textit{Notes:}  Sandwich standard errors are reported within parentheses. One observation corresponds to one participant. \phantom{h} \hfill {$^{*}$p$<$0.1; $^{**}$p$<$0.05; $^{***}$p$<$0.01} }}}\\ 
\end{tabular} 
\end{table}

\begin{table}[H] \centering 
  \caption{Regression results relative of OLS to estimate the impact of the interventions on participants' agreement fraction, switch fraction, and mean influence, evaluated only on cases characterized by high predictive uncertainty.} 
  \label{} 
\begin{tabular}{@{\extracolsep{5pt}}lD{.}{.}{-3} D{.}{.}{-3} D{.}{.}{-3} } 
\\[-1.8ex]\hline 
\hline \\[-1.8ex] 
 & \multicolumn{3}{c}{\textit{Dependent variable:}} \\ 
\cline{2-4} 
\\[-1.8ex] & \multicolumn{1}{c}{Agreement fraction} & \multicolumn{1}{c}{Switch fraction} & \multicolumn{1}{c}{Mean influence} \\ 
\\[-1.8ex] & \multicolumn{1}{c}{(1)} & \multicolumn{1}{c}{(2)} & \multicolumn{1}{c}{(3)}\\ 
\hline \\[-1.8ex] 
 \textit{Medium agreement} & 0.074^{**} & 0.154^{***} & 0.128^{**} \\ 
  & (0.037) & (0.055) & (0.054) \\ 
   \textit{High agreement} & 0.037 & 0.096^{*} & 0.141^{**} \\ 
  & (0.035) & (0.051) & (0.065) \\ 
  \textit{Medium agreement} $\times$ \textit{feedback} & -0.079^{**} & -0.181^{***} & -0.170^{***} \\ 
  & (0.040) & (0.060) & (0.061) \\ 
  \textit{High agreement} $\times$ \textit{feedback} & -0.048 & -0.097 & -0.074 \\ 
  & (0.041) & (0.060) & (0.073) \\ 
  \textit{Neutral incentives} & 0.012 & 0.028 & 0.049 \\ 
  & (0.029) & (0.042) & (0.047) \\ 
  \textit{High-TP incentives} & 0.001 & 0.004 & 0.020 \\ 
  & (0.028) & (0.042) & (0.048) \\ 
  \textit{Intercept} & 0.614^{***} & 0.316^{***} & 0.295^{***} \\ 
  & (0.026) & (0.037) & (0.043) \\ 
 \hline \\[-1.8ex] 
Observations & \multicolumn{1}{c}{493} & \multicolumn{1}{c}{493} & \multicolumn{1}{c}{493} \\ 
R$^{2}$ & \multicolumn{1}{c}{0.014} & \multicolumn{1}{c}{0.031} & \multicolumn{1}{c}{0.029} \\ 
Adjusted R$^{2}$ & \multicolumn{1}{c}{0.002} & \multicolumn{1}{c}{0.019} & \multicolumn{1}{c}{0.017} \\ 
Residual Std. Error (df = 486) & \multicolumn{1}{c}{0.264} & \multicolumn{1}{c}{0.386} & \multicolumn{1}{c}{0.428} \\ 
\hline 
\hline \\[-1.8ex] 
\multicolumn{4}{l}{\footnotesize{\textit{Note:} Sandwich standard errors are reported within parentheses. \hfill {$^{*}$p$<$0.1; $^{**}$p$<$0.05; $^{***}$p$<$0.01} }}\\ 
\end{tabular} 
\end{table}

\begin{table}[H] \centering 
  \caption{Regression results relative of OLS to estimate impact of the interventions on participants' agreement fraction, switch fraction, and mean influence, evaluated only on cases where participants reported levels of confidence equal or lower than 3 (out of 5).} 
  \label{} 
\begin{tabular}{@{\extracolsep{5pt}}lD{.}{.}{-3} D{.}{.}{-3} D{.}{.}{-3} } 
\\[-1.8ex]\hline 
\hline \\[-1.8ex] 
 & \multicolumn{3}{c}{\textit{Dependent variable:}} \\ 
\cline{2-4} 
\\[-1.8ex] & \multicolumn{1}{c}{Agreement fraction} & \multicolumn{1}{c}{Switch fraction} & \multicolumn{1}{c}{Mean influence} \\ 
\\[-1.8ex] & \multicolumn{1}{c}{(1)} & \multicolumn{1}{c}{(2)} & \multicolumn{1}{c}{(3)}\\ 
\hline \\[-1.8ex] 
 \textit{Medium agreement} & 0.007 & 0.128 & 0.021 \\ 
  & (0.052) & (0.091) & (0.072) \\ 
   \textit{High agreement} & 0.070 & 0.158 & 0.132 \\ 
  & (0.047) & (0.102) & (0.113) \\ 
  \textit{Medium agreement} $\times$ \textit{feedback} & 0.011 & -0.080 & -0.023 \\ 
  & (0.059) & (0.105) & (0.091) \\ 
  \textit{High agreement} $\times$ \textit{feedback} & -0.033 & -0.128 & -0.126 \\ 
  & (0.051) & (0.118) & (0.124) \\ 
  \textit{Neutral incentives} & 0.045 & -0.022 & 0.101 \\ 
  & (0.042) & (0.076) & (0.072) \\ 
  \textit{High-TP incentives} & 0.014 & -0.074 & 0.067 \\ 
  & (0.039) & (0.075) & (0.070) \\ 
  \textit{Intercept} & 0.734^{***} & 0.420^{***} & 0.281^{***} \\ 
  & (0.037) & (0.065) & (0.063) \\ 
 \hline \\[-1.8ex] 
Observations & \multicolumn{1}{c}{168} & \multicolumn{1}{c}{167} & \multicolumn{1}{c}{168} \\ 
R$^{2}$ & \multicolumn{1}{c}{0.021} & \multicolumn{1}{c}{0.029} & \multicolumn{1}{c}{0.028} \\ 
Adjusted R$^{2}$ & \multicolumn{1}{c}{-0.016} & \multicolumn{1}{c}{-0.008} & \multicolumn{1}{c}{-0.008} \\ 
Residual Std. Error & \multicolumn{1}{c}{0.213 (df = 161)} & \multicolumn{1}{c}{0.399 (df = 160)} & \multicolumn{1}{c}{0.369 (df = 161)} \\ 
\hline 
\hline \\[-1.8ex] 
\multicolumn{4}{l}{\footnotesize{\textit{Note:} Sandwich standard errors are reported within parentheses. \hfill {$^{*}$p$<$0.1; $^{**}$p$<$0.05; $^{***}$p$<$0.01} }}\\ 
\end{tabular} 
\end{table}

\begin{table}[H] \centering 
  \caption{Regression results relative of OLS to estimate the impact of the interventions on participants' perceived utility (first questionnaire) and self-reported level of trust (second questionnaire) in the AI model.} 
  \label{} 
\begin{tabular}{@{\extracolsep{5pt}}lD{.}{.}{-3} D{.}{.}{-3} } 
\\[-1.8ex]\hline 
\hline \\[-1.8ex] 
 & \multicolumn{2}{c}{\textit{Dependent variable:}} \\ 
\cline{2-3} 
\\[-1.8ex] & \multicolumn{1}{c}{Perceived utility} & \multicolumn{1}{c}{Trust} \\ 
\\[-1.8ex] & \multicolumn{1}{c}{(1)} & \multicolumn{1}{c}{(2)}\\ 
\hline \\[-1.8ex] 
 \textit{Medium agreement} & 0.221 & 0.002 \\ 
  & (0.142) & (0.127) \\ 
   \textit{High agreement} & 0.248 & 0.074 \\ 
  & (0.154) & (0.117) \\ 
  \textit{Medium agreement} $\times$ \textit{feedback} & -0.331^{*} & -0.060 \\ 
  & (0.181) & (0.151) \\ 
  \textit{High agreement} $\times$ \textit{feedback} & -0.322 & 0.014 \\ 
  & (0.212) & (0.143) \\ 
  \textit{Neutral incentives} & 0.109 & 0.111 \\ 
  & (0.134) & (0.104) \\ 
  \textit{High-TP incentives} & -0.095 & 0.055 \\ 
  & (0.132) & (0.100) \\ 
  \textit{Intercept} & 5.330^{***} & 5.221^{***} \\ 
  & (0.111) & (0.089) \\ 
 \hline \\[-1.8ex] 
Observations & \multicolumn{1}{c}{493} & \multicolumn{1}{c}{493} \\ 
R$^{2}$ & \multicolumn{1}{c}{0.019} & \multicolumn{1}{c}{0.005} \\ 
Adjusted R$^{2}$ & \multicolumn{1}{c}{0.007} & \multicolumn{1}{c}{-0.007} \\ 
Residual Std. Error (df = 486) & \multicolumn{1}{c}{1.208} & \multicolumn{1}{c}{0.931} \\ 
\hline 
\hline \\[-1.8ex] 
\multicolumn{3}{l} {\parbox[t]{0.8\textwidth}{\footnotesize{ \textit{Notes:} Sandwich standard errors are reported within parentheses. Answers were measured on a 7-point Likert scale and converted into scores ranging from 1 to 7. More details about the questions are contained in Section \ref{sec:procedure}.}}} \\ \multicolumn{3}{r}{\footnotesize{$^{*}$p$<$0.1; $^{**}$p$<$0.05; $^{***}$p$<$0.01}} \\
\end{tabular} 
\end{table}

\begin{table}[H] \centering 
  \caption{Regression results relative of OLS to estimate the impact of the interventions on the participants' share of positive predictions made before seeing the AI's recommendation.} 
  \label{} 
\begin{tabular}{@{\extracolsep{5pt}}lD{.}{.}{-3} D{.}{.}{-3} D{.}{.}{-3} } 
\\[-1.8ex]\hline 
\hline \\[-1.8ex] 
 & \multicolumn{3}{c}{\textit{Cases considered:}} \\ 
\cline{2-4} 
\\[-1.8ex] & \multicolumn{1}{c}{All cases} & \multicolumn{1}{c}{High predictive uncertainty} & \multicolumn{1}{c}{Low confidence} \\ 
\\[-1.8ex] & \multicolumn{1}{c}{(1)} & \multicolumn{1}{c}{(2)} & \multicolumn{1}{c}{(3)}\\ 
\hline \\[-1.8ex] 
 \textit{Medium agreement} & 0.030 & 0.027 & 0.099^{*} \\ 
  & (0.030) & (0.037) & (0.054) \\ 
   \textit{High agreement} & 0.016 & 0.049 & 0.021 \\ 
  & (0.030) & (0.038) & (0.048) \\ 
  \textit{Medium agreement} $\times$ \textit{feedback} & 0.006 & -0.003 & -0.100 \\ 
  & (0.036) & (0.043) & (0.068) \\ 
  \textit{High agreement} $\times$ \textit{feedback} & -0.035 & -0.072 & -0.064 \\ 
  & (0.036) & (0.046) & (0.058) \\ 
  \textit{Neutral incentives} & -0.017 & 0.012 & -0.017 \\ 
  & (0.027) & (0.032) & (0.044) \\ 
  \textit{High-TP incentives} & -0.020 & 0.003 & 0.002 \\ 
  & (0.025) & (0.031) & (0.044) \\ 
  \textit{Intercept} & 0.581^{***} & 0.622^{***} & 0.459^{***} \\ 
  & (0.024) & (0.028) & (0.038) \\ 
 \hline \\[-1.8ex] 
Observations & \multicolumn{1}{c}{493} & \multicolumn{1}{c}{493} & \multicolumn{1}{c}{168} \\ 
R$^{2}$ & \multicolumn{1}{c}{0.008} & \multicolumn{1}{c}{0.007} & \multicolumn{1}{c}{0.036} \\ 
Adjusted R$^{2}$ & \multicolumn{1}{c}{-0.005} & \multicolumn{1}{c}{-0.005} & \multicolumn{1}{c}{0.0004} \\ 
Residual Std. Error & \multicolumn{1}{c}{0.234 (df = 486)} & \multicolumn{1}{c}{0.288 (df = 486)} & \multicolumn{1}{c}{0.232 (df = 161)} \\ 
\hline 
\hline \\[-1.8ex] 
\multicolumn{4}{l} {\parbox[t]{0.8\textwidth}{\footnotesize{ \textit{Notes:} Sandwich standard errors are reported within parentheses.  }}} \\ \multicolumn{4}{r}{\footnotesize{$^{*}$p$<$0.1; $^{**}$p$<$0.05; $^{***}$p$<$0.01}} \\
\end{tabular} 
\end{table}

\begin{table}[H] \centering 
  \caption{Regression results relative of OLS to estimate the impact of the interventions on the participants' self-reported levels of confidence for the cases (mean for each participant) and the two questionnaires.}  
  \label{} 
\begin{tabular}{@{\extracolsep{5pt}}lD{.}{.}{-3} D{.}{.}{-3} D{.}{.}{-3} } 
\\[-1.8ex]\hline 
\hline \\[-1.8ex] 
 & \multicolumn{3}{c}{\textit{Dependent variable: confidence measured in}} \\ 
\cline{2-4} 
\\[-1.8ex] & \multicolumn{1}{c}{Cases} & \multicolumn{1}{c}{First questionnaire} & \multicolumn{1}{c}{Second questionnaire} \\ 
\\[-1.8ex] & \multicolumn{1}{c}{(1)} & \multicolumn{1}{c}{(2)} & \multicolumn{1}{c}{(3)}\\ 
\hline \\[-1.8ex] 
\textit{Medium agreement} & 0.130^{*} & 0.331^{***} & 0.177^{*} \\ 
  & (0.075) & (0.105) & (0.106) \\ 
   \textit{High agreement} & 0.256^{***} & 0.505^{***} & 0.236^{**} \\ 
  & (0.083) & (0.110) & (0.103) \\ 
  \textit{Medium agreement} $\times$ \textit{feedback} & -0.132 & -0.230^{*} & -0.290^{**} \\ 
  & (0.100) & (0.129) & (0.131) \\ 
  \textit{High agreement} $\times$ \textit{feedback} & -0.272^{**} & -0.353^{**} & -0.079 \\ 
  & (0.112) & (0.146) & (0.136) \\ 
  \textit{Neutral incentives} & -0.116 & 0.023 & 0.055 \\ 
  & (0.071) & (0.097) & (0.094) \\ 
  \textit{High-TP incentives} & -0.023 & -0.033 & -0.039 \\ 
  & (0.072) & (0.093) & (0.090) \\ 
  \textit{Intercept} & 3.595^{***} & 3.555^{***} & 3.826^{***} \\ 
  & (0.061) & (0.084) & (0.080) \\ 
 \hline \\[-1.8ex] 
Observations & \multicolumn{1}{c}{493} & \multicolumn{1}{c}{493} & \multicolumn{1}{c}{493} \\ 
R$^{2}$ & \multicolumn{1}{c}{0.029} & \multicolumn{1}{c}{0.046} & \multicolumn{1}{c}{0.024} \\ 
Adjusted R$^{2}$ & \multicolumn{1}{c}{0.017} & \multicolumn{1}{c}{0.035} & \multicolumn{1}{c}{0.012} \\ 
Residual Std. Error (df = 486) & \multicolumn{1}{c}{0.643} & \multicolumn{1}{c}{0.860} & \multicolumn{1}{c}{0.847} \\ 
\hline 
\hline \\[-1.8ex] 
\multicolumn{4}{l} {\parbox[t]{0.98\textwidth}{\footnotesize{ \textit{Notes:} Sandwich standard errors are reported within parentheses. ``Cases'' refers to the level of confidence in the predictions that participants reported for each of the cases. ``First questionnaire'' and ``Second questionnaire'' refer to the questions about confidence elicited in the first and second questionnaires. The 5-point Likert scales on which the two types of outcomes were elicited are different (see Section \ref{sec:experiment}).}}} \\ \multicolumn{4}{r}{\footnotesize{$^{*}$p$<$0.1; $^{**}$p$<$0.05; $^{***}$p$<$0.01}} \\
\end{tabular} 
\end{table}

\begin{figure}
    \centering
    \includegraphics[width=0.9\textwidth]{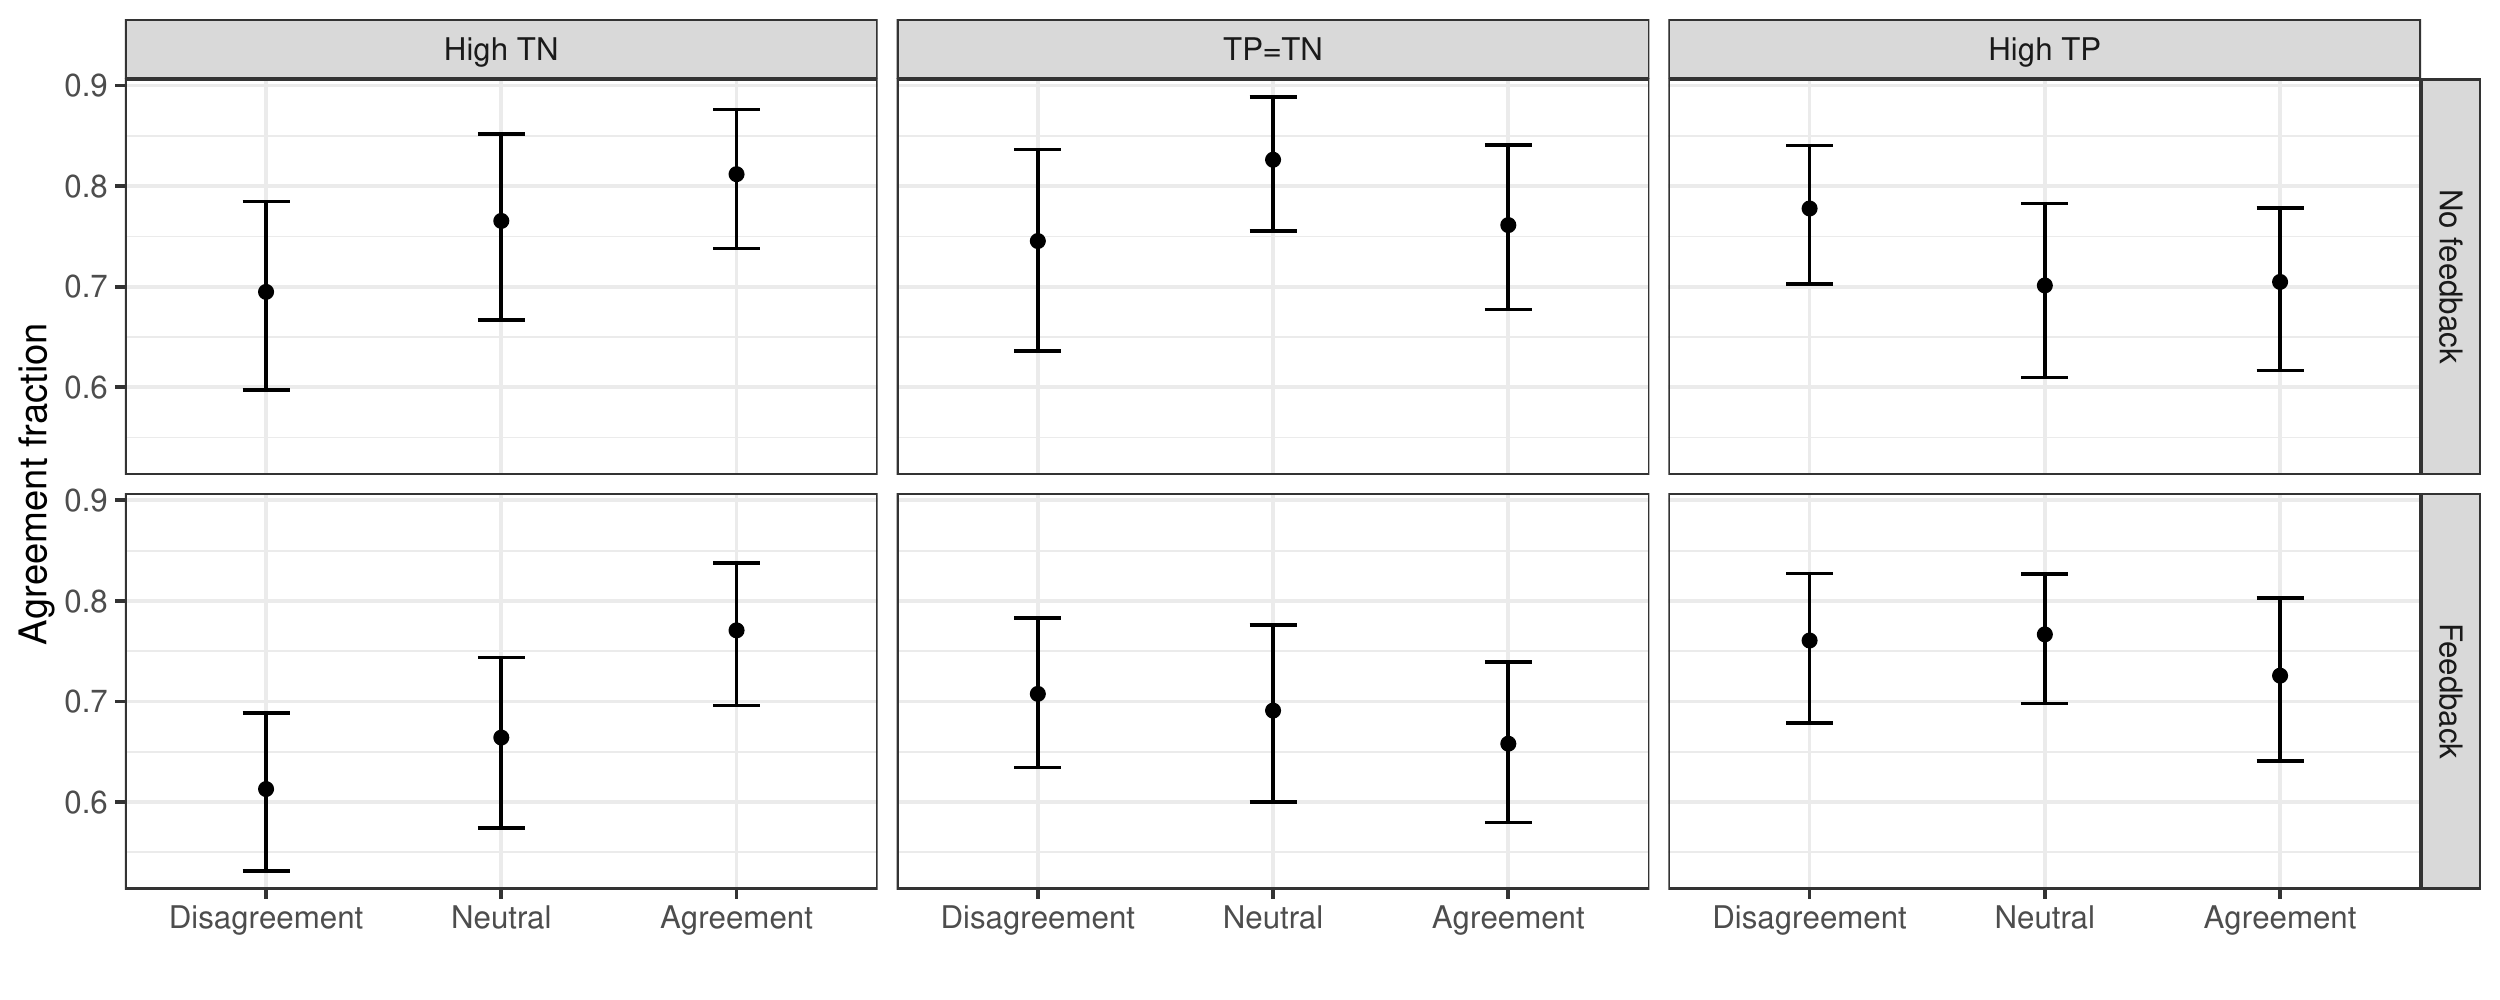}
    \includegraphics[width=0.9\textwidth]{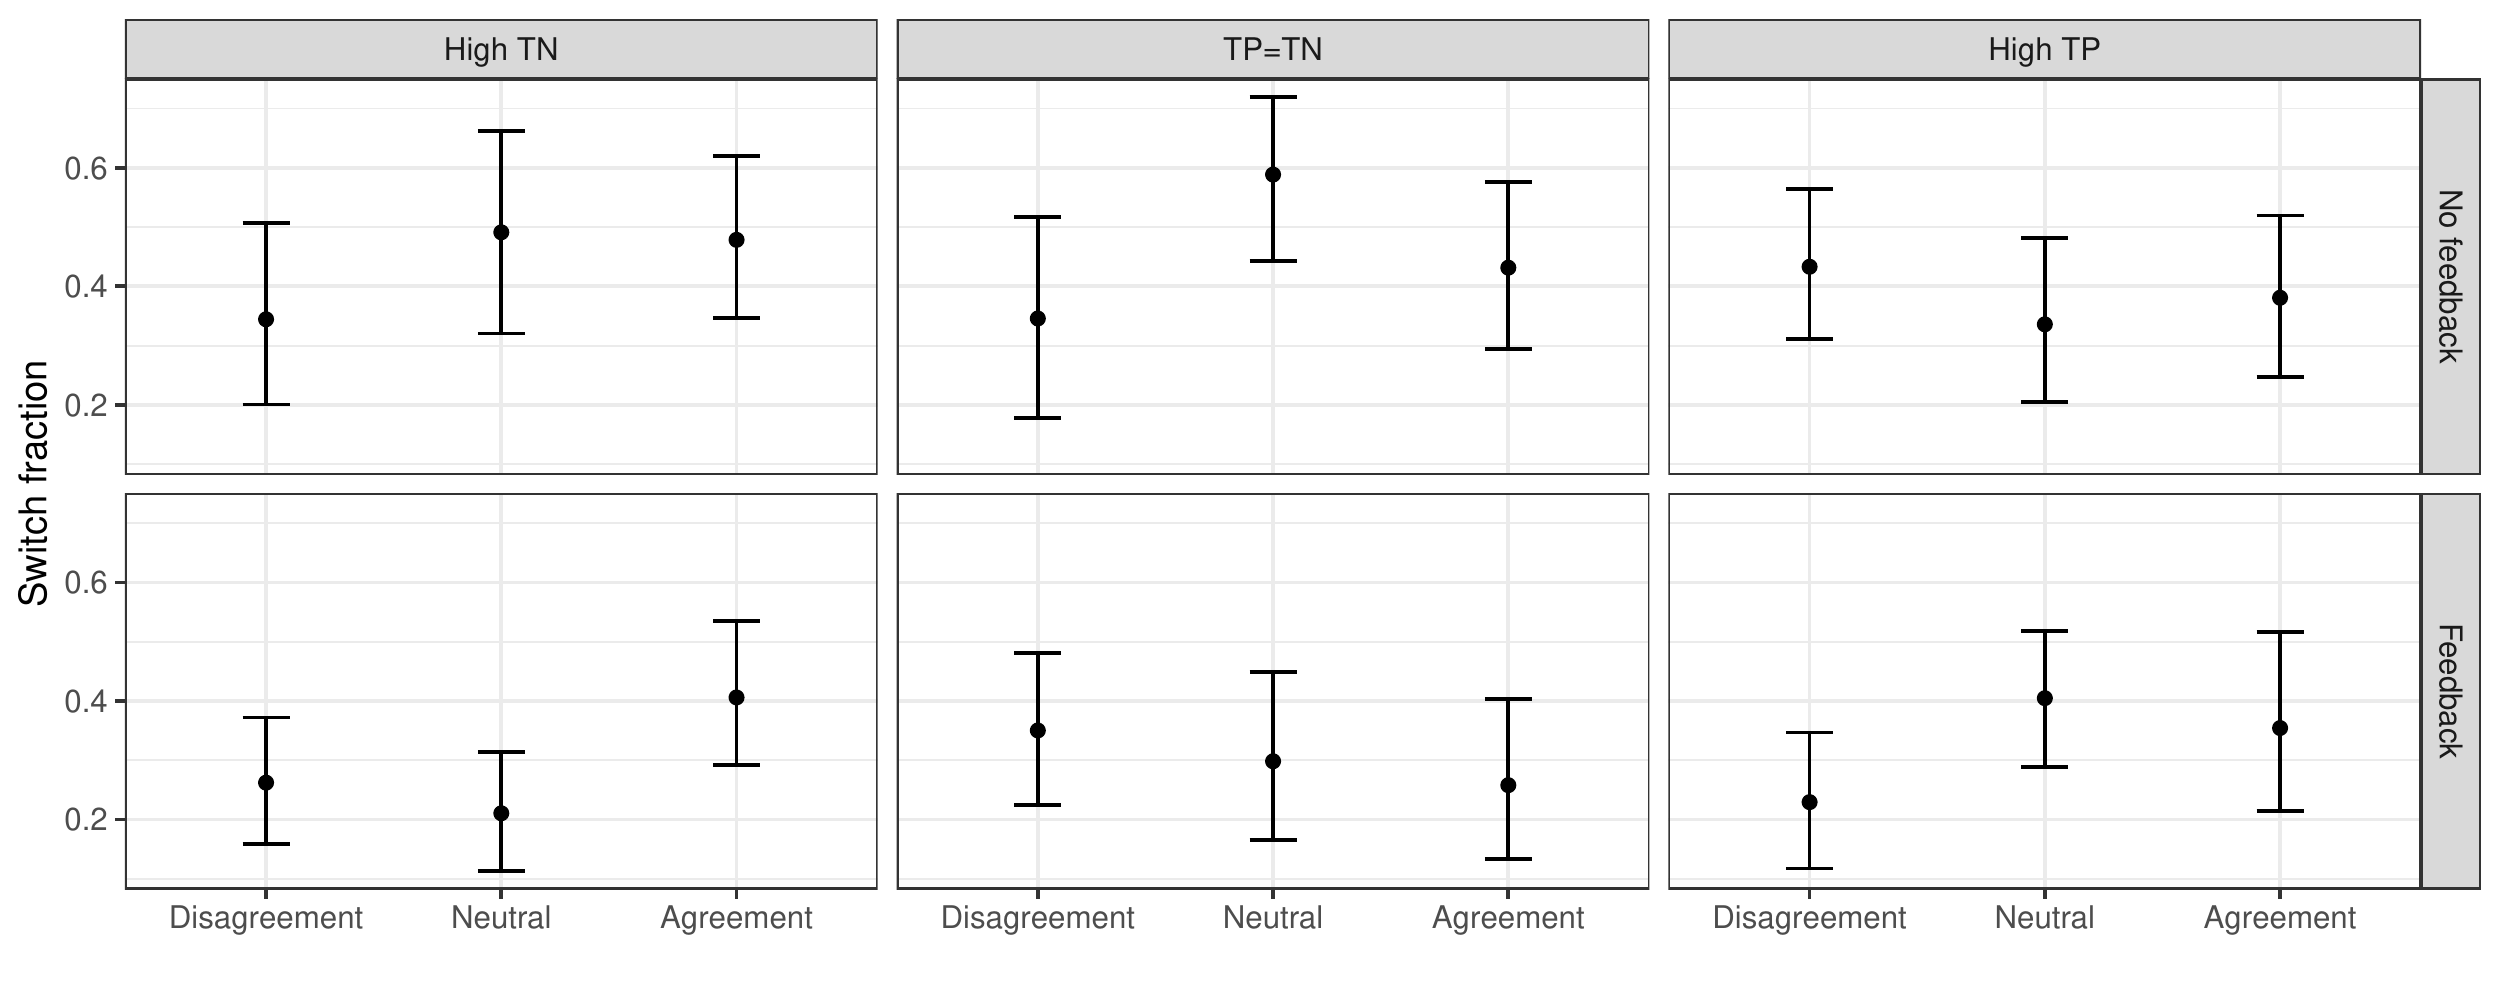}
  \includegraphics[width=0.9\textwidth]{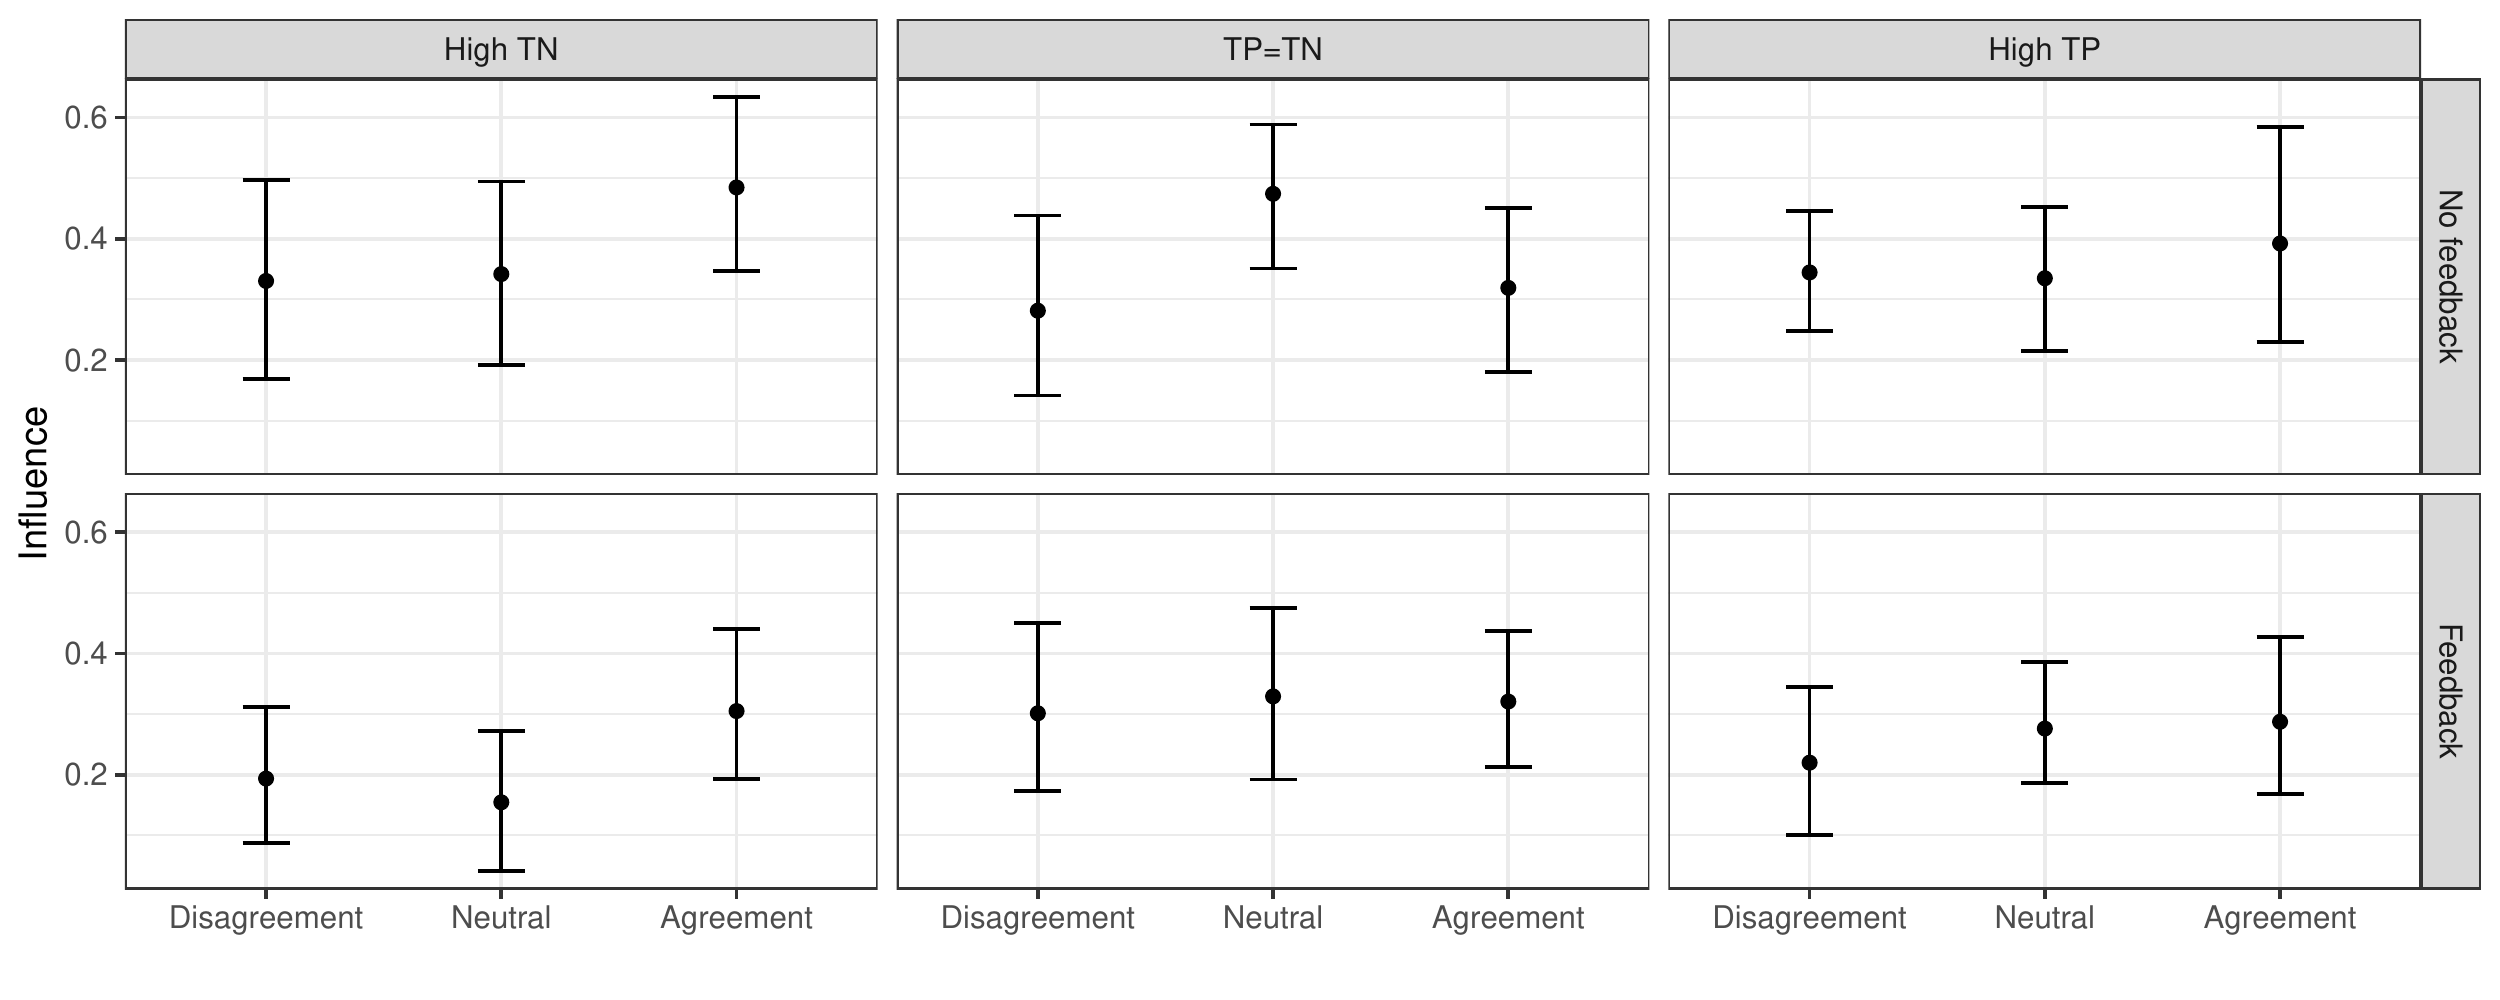}
    \caption{Agreement fraction (top), switch fraction (middle), and mean influence (bottom) for participants' predictions in the second phase of the survey across the agreement (horizontal axis), incentives (panels, label on the top), and feedback (label on the right) interventions. Dots and vertical bars correspond to the mean estimates and 95\% confidence intervals for the mean computed via percentile bootstrap, respectively.}
    \label{fig:outcome_metrics_reliance_alternative}
\end{figure}

\newpage

\section{Additional information on survey}\label{sec:app_moreinfosurvey}

\begin{figure}[h]
\includegraphics[width=0.8\textwidth]{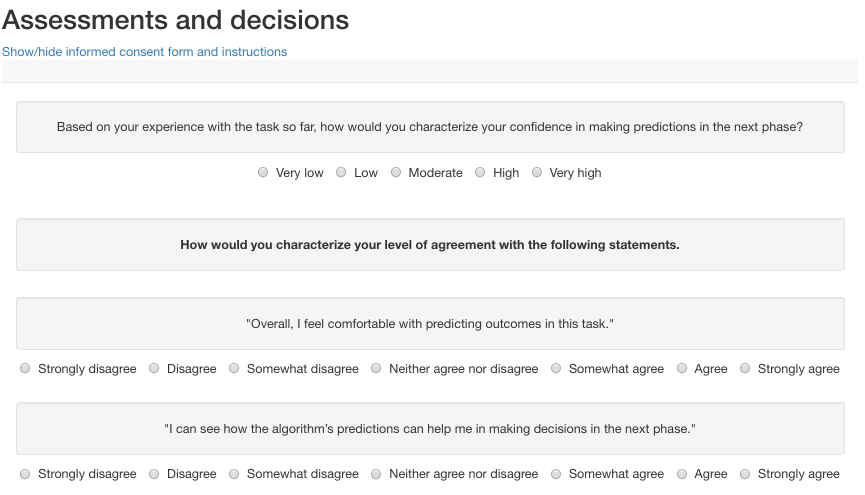}
\caption{Screenshot of the questions contained in the first questionnaire.}
\end{figure}

\begin{figure}[h]
\includegraphics[width=0.8\textwidth]{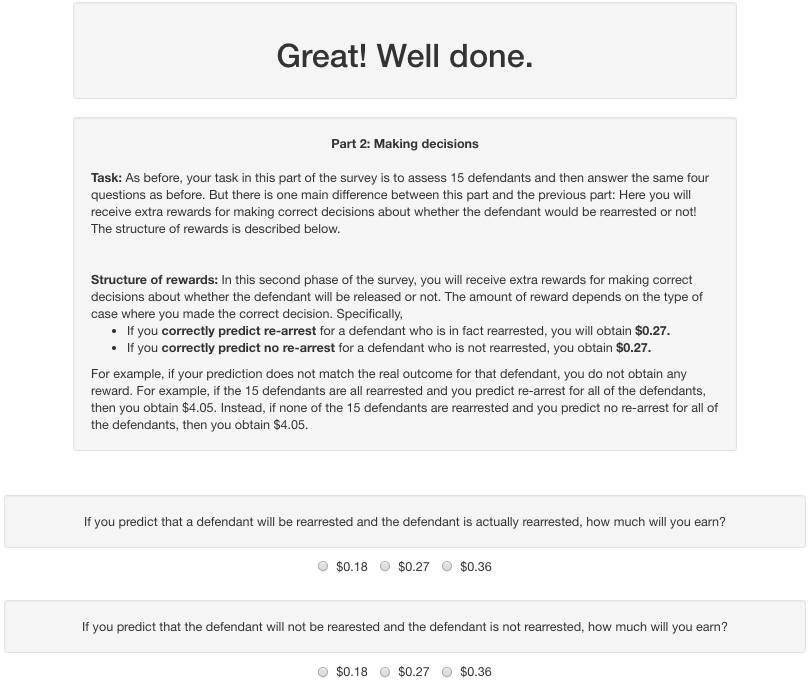}
\caption{Screenshot of the instructions about the incentives structure that were shown before the second phase of the survey. The participant was allowed to proceed only once they had correctly answered the two questions.}
\end{figure}

\begin{figure}[h]
\includegraphics[width=0.8\textwidth]{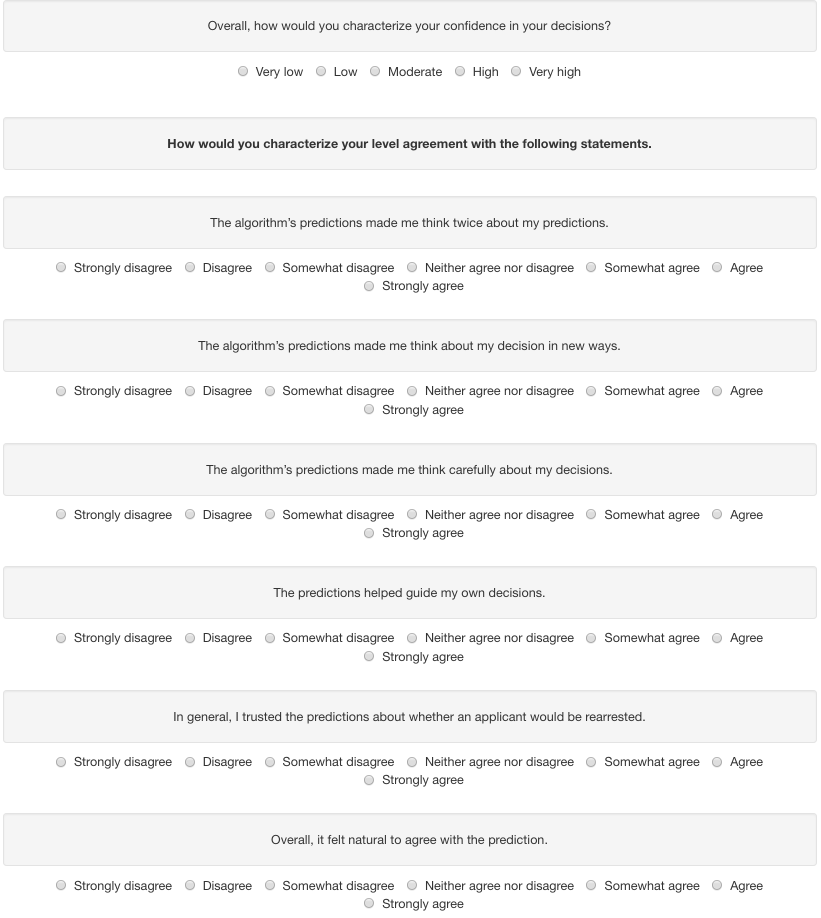}
\caption{Screenshot of the questions on confidence and trust in the AI tool contained in the second questionnaire.}
\end{figure}

\begin{figure}[h]
\includegraphics[width=0.8\textwidth]{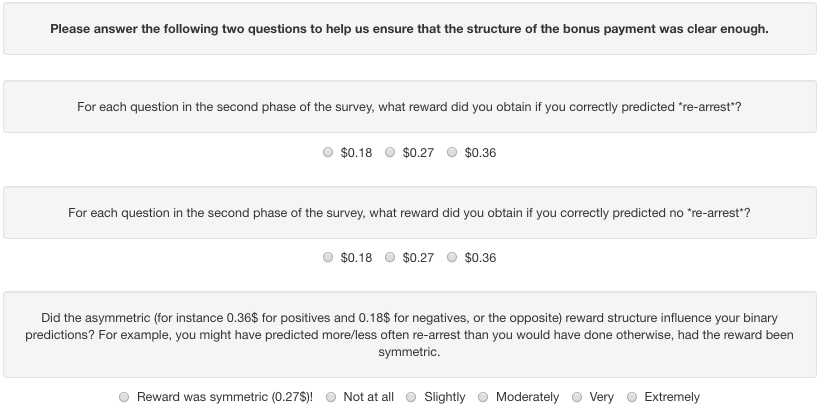}
\caption{Screenshot of the questions on the incentives structure contained in the second questionnaire.}
\end{figure}
